# Supplementary material for: Textualize Visual Prompt for Image Editing via Diffusion Bridge
Source: arXiv:2501.03495 source file (2025-01-27)
Supplement: Supplementary file 1 [file supp_checklist.tex]

\clearpage
\section{Reproducibility Checklist}
This paper:

\noindent 1. Includes a conceptual outline and/or pseudocode description of AI methods introduced (yes)

\noindent 2. Clearly delineates statements that are opinions, hypothesis, and speculation from objective facts and results (yes)

\noindent 3. Provides well marked pedagogical references for less-familiare readers to gain background necessary to replicate the paper (yes)

\noindent 4. Does this paper make theoretical contributions? (no)

\noindent If yes, please complete the list below.

\noindent 5. All assumptions and restrictions are stated clearly and formally. (yes/partial/no)

\noindent 6. All novel claims are stated formally (e.g., in theorem statements). (yes/partial/no)

\noindent 7. Proofs of all novel claims are included. (yes/partial/no)

\noindent 8. Proof sketches or intuitions are given for complex and/or novel results. (yes/partial/no)

\noindent Appropriate citations to theoretical tools used are given. (yes/partial/no)

\noindent 9. All theoretical claims are demonstrated empirically to hold. (yes/partial/no/NA)

\noindent 10. All experimental code used to eliminate or disprove claims is included. (NA)

\noindent 11. Does this paper rely on one or more datasets? (no)

\noindent If yes, please complete the list below.

\noindent 12. A motivation is given for why the experiments are conducted on the selected datasets (NA)

\noindent 13. All novel datasets introduced in this paper are included in a data appendix. (NA)

\noindent 14. All novel datasets introduced in this paper will be made publicly available upon publication of the paper with a license that allows free usage for research purposes. (NA)

\noindent 15. All datasets drawn from the existing literature (potentially including authors’ own previously published work) are accompanied by appropriate citations. (yes)

\noindent 16. All datasets drawn from the existing literature (potentially including authors’ own previously published work) are publicly available. (yes)

\noindent 17. All datasets that are not publicly available are described in detail, with explanation why publicly available alternatives are not scientifically satisficing. (yes)

\noindent 18. Does this paper include computational experiments? (yes)

\noindent If yes, please complete the list below.

\noindent 19. Any code required for pre-processing data is included in the appendix. (NA).

\noindent 20. All source code required for conducting and analyzing the experiments is included in a code appendix. (no)

\noindent 21. All source code required for conducting and analyzing the experiments will be made publicly available upon publication of the paper with a license that allows free usage for research purposes. (yes)

\noindent 22. All source code implementing new methods have comments detailing the implementation, with references to the paper where each step comes from (yes)

\noindent 23. If an algorithm depends on randomness, then the method used for setting seeds is described in a way sufficient to allow replication of results. (yes)

\noindent 24. This paper specifies the computing infrastructure used for running experiments (hardware and software), including GPU/CPU models; amount of memory; operating system; names, and versions of relevant software libraries and frameworks. (yes)

\noindent 25. This paper formally describes the evaluation metrics used and explains the motivation for choosing these metrics. (yes)

\noindent 26. This paper states the number of algorithm runs used to compute each reported result. (yes)

\noindent 27. Analysis of experiments goes beyond single-dimensional summaries of performance (e.g., average; median) to include measures of variation, confidence, or other distributional information. (yes)

\noindent 28. The significance of any improvement or decrease in performance is judged using appropriate statistical tests (e.g., Wilcoxon signed-rank). (yes)

\noindent 29. This paper lists all final (hyper-)parameters used for each model/algorithm in the paper’s experiments. (yes)

\noindent 30. This paper states the number and range of values tried per (hyper-) parameter during the development of the paper, along with the criterion used for selecting the final parameter setting. (yes)
